# Supplementary material for: Introduction to String Theory
Source: arXiv:2311.18111 source file (2024-01-14)
Supplement: Supplementary file 1 [file Exercises_solutions.tex]

\chapter{Exercises Solutions}
\label{app:Exercises_Solutions}

%%%%%%%%%%%%%%%%%%%%%%%%%%%%%%%%%%%%%%%%%%%%%%%%%%%%%%%%%%%%%%%%%%%%%%%%%%%%%%%%%%%%%%%%%%%%%%%%%%%%%%%%%%%%%%%%%%%%%%%%%%%%%%%%%%%%%%%%%%%%%%%%%%%%%%%%%%%%%%%%%%%%%%%%%%%%
%%%%%%%%%%%%%%%%%%%%%%%%%%%%%%%%%%%%%%%%%%%%%%%%%%%%%%%%%%%%%%%%%%%%%%%%%%%%%%%%%%%%%%%%%%%%%%%%%%%%%%%%%%%%%%%%%%%%%%%%%%%%%%%%%%%%%%%%%%%%%%%%%%%%%%%%%%%%%%%%%%%%%%%%%%%%
\section{Solutions to exercises from chapter 2}
\paragraph{Exercise \ref{exer:free_part_gauge_transf} (page \pageref{exer:free_part_gauge_transf})}\mbox{}\\
\paragraph{Exercise \ref{exer:free_part_gauge_transf_leave_S_unchanged} (page \pageref{exer:free_part_gauge_transf_leave_S_unchanged})}\mbox{}\\
\paragraph{Exercise \ref{exer:free_part_theta_tau} (page \pageref{exer:free_part_theta_tau})}\mbox{}\\

%%%%%%%%%%%%%%%%%%%%%%%%%%%%%%%%%%%%%%%%%%%%%%%%%%%%%%%%%%%%%%%%%%%%%%%%%%%%%%%%%%%%%%%%%%%%%%%%%%%%%%%%%%%%%%%%%%%%%%%%%%%%%%%%%%%%%%%%%%%%%%%%%%%%%%%%%%%%%%%%%%%%%%%%%%%%
%%%%%%%%%%%%%%%%%%%%%%%%%%%%%%%%%%%%%%%%%%%%%%%%%%%%%%%%%%%%%%%%%%%%%%%%%%%%%%%%%%%%%%%%%%%%%%%%%%%%%%%%%%%%%%%%%%%%%%%%%%%%%%%%%%%%%%%%%%%%%%%%%%%%%%%%%%%%%%%%%%%%%%%%%%%%
%%%%%%%%%%%%%%%%%%%%%%%%%%%%%%%%%%%%%%%%%%%%%%%%%%%%%%%%%%%%%%%%%%%%%%%%%%%%%%%%%%%%%%%%%%%%%%%%%%%%%%%%%%%%%%%%%%%%%%%%%%%%%%%%%%%%%%%%%%%%%%%%%%%%%%%%%%%%%%%%%%%%%%%%%%%%
\section{Solutions to exercises from chapter 3}
\paragraph{Exercise \ref{exer:quantization_closed_string} (page \pageref{exer:quantization_closed_string})}\mbox{}\\
\paragraph{Exercise \ref{exer:virasoro_operators} (page \pageref{exer:virasoro_operators})}\mbox{}\\
\paragraph{Exercise \ref{exer:commutator_virasoro_operator_and_oscillator} (page \pageref{exer:commutator_virasoro_operator_and_oscillator})}\mbox{}\\
\paragraph{Exercise \ref{exer:closed_OCQ_N=2} (page \pageref{exer:closed_OCQ_N=2})}\mbox{}\\
\paragraph{Exercise \ref{exer:Neumann_BC} (page \pageref{exer:Neumann_BC})}\mbox{}\\
\paragraph{Exercise \ref{exer:ND_string} (page \pageref{exer:ND_string})}\mbox{}\\
\paragraph{Exercise \ref{exer:ND_string_stressenergy_tensor} (page \pageref{exer:ND_string_stressenergy_tensor})}\mbox{}\\
\paragraph{Exercise \ref{exer:find_coeff_suchthat_state_is_physical} (page \pageref{exer:find_coeff_suchthat_state_is_physical})}\mbox{}\\
\paragraph{Exercise \ref{exer:generic_N=2_open_string_state} (page \pageref{exer:generic_N=2_open_string_state})}\mbox{}\\

%%%%%%%%%%%%%%%%%%%%%%%%%%%%%%%%%%%%%%%%%%%%%%%%%%%%%%%%%%%%%%%%%%%%%%%%%%%%%%%%%%%%%%%%%%%%%%%%%%%%%%%%%%%%%%%%%%%%%%%%%%%%%%%%%%%%%%%%%%%%%%%%%%%%%%%%%%%%%%%%%%%%%%%%%%%%
%%%%%%%%%%%%%%%%%%%%%%%%%%%%%%%%%%%%%%%%%%%%%%%%%%%%%%%%%%%%%%%%%%%%%%%%%%%%%%%%%%%%%%%%%%%%%%%%%%%%%%%%%%%%%%%%%%%%%%%%%%%%%%%%%%%%%%%%%%%%%%%%%%%%%%%%%%%%%%%%%%%%%%%%%%%%
%%%%%%%%%%%%%%%%%%%%%%%%%%%%%%%%%%%%%%%%%%%%%%%%%%%%%%%%%%%%%%%%%%%%%%%%%%%%%%%%%%%%%%%%%%%%%%%%%%%%%%%%%%%%%%%%%%%%%%%%%%%%%%%%%%%%%%%%%%%%%%%%%%%%%%%%%%%%%%%%%%%%%%%%%%%%
\section{Solutions to exercises from chapter 4}
\paragraph{Exercise \ref{exer:primary_field_expansion_and_residue_theorem} (page \pageref{exer:primary_field_expansion_and_residue_theorem})}\mbox{}\\
\paragraph{Exercise \ref{exer:ln_algebra} (page \pageref{exer:ln_algebra})}\mbox{}\\
\paragraph{Exercise \ref{exer:comm_delta_epsilon} (page \pageref{exer:comm_delta_epsilon})}\mbox{}\\
\paragraph{Exercise \ref{exer:OPE_TT} (page \pageref{exer:OPE_TT})}\mbox{}\\
\paragraph{Exercise \ref{exer:Virasoro_algebra_CFT} (page \pageref{exer:Virasoro_algebra_CFT})}\mbox{}\\
\paragraph{Exercise \ref{exer:Ln_commutators_with_phi_and_phin} (page \pageref{exer:Ln_commutators_with_phi_and_phin})}\mbox{}\\
\paragraph{Exercise \ref{exer:delta_epsilon_T} (page \pageref{exer:delta_epsilon_T})}\mbox{}\\
\paragraph{Exercise \ref{exer:BPZ_conjugation} (page \pageref{exer:BPZ_conjugation})}\mbox{}\\
\paragraph{Exercise \ref{exer:Virasoro_constraint_CFT} (page \pageref{exer:Virasoro_constraint_CFT})}\mbox{}\\
\paragraph{Exercise \ref{exer:generic-3_points_function} (page \pageref{exer:generic-3_points_function})}\mbox{}\\
\paragraph{Exercise \ref{exer:OPE_jj} (page \pageref{exer:OPE_jj})}\mbox{}\\
\paragraph{Exercise \ref{exer:OPE_T_planewave} (page \pageref{exer:OPE_T_planewave})}\mbox{}\\
\paragraph{Exercise \ref{exer:OPE_T_stateN=1} (page \pageref{exer:OPE_T_stateN=1})}\mbox{}\\
\paragraph{Exercise \ref{exer:OPE_T_b_c} (page \pageref{exer:OPE_T_b_c})}\mbox{}\\
\paragraph{Exercise \ref{exer:OPE_T_T_ghost} (page \pageref{exer:OPE_T_T_ghost})}\mbox{}\\
\paragraph{Exercise \ref{exer:corr_func_ccc} (page \pageref{exer:corr_func_ccc})}\mbox{}\\
\paragraph{Exercise \ref{exer:comm_Q_X} (page \pageref{exer:comm_Q_X})}\mbox{}\\
\paragraph{Exercise \ref{exer:comm_Q_c} (page \pageref{exer:comm_Q_c})}\mbox{}\\
\paragraph{Exercise \ref{exer:Q_nilpotent} (page \pageref{exer:Q_nilpotent})}\mbox{}\\
\paragraph{Exercise \ref{exer:comm_Q_j_gh} (page \pageref{exer:comm_Q_j_gh})}\mbox{}\\
\paragraph{Exercise \ref{exer:comm_Q_V} (page \pageref{exer:comm_Q_V})}\mbox{}\\
\paragraph{Exercise \ref{exer:open_string_corr_func} (page \pageref{exer:open_string_corr_func})}\mbox{}\\

%%%%%%%%%%%%%%%%%%%%%%%%%%%%%%%%%%%%%%%%%%%%%%%%%%%%%%%%%%%%%%%%%%%%%%%%%%%%%%%%%%%%%%%%%%%%%%%%%%%%%%%%%%%%%%%%%%%%%%%%%%%%%%%%%%%%%%%%%%%%%%%%%%%%%%%%%%%%%%%%%%%%%%%%%%%%
%%%%%%%%%%%%%%%%%%%%%%%%%%%%%%%%%%%%%%%%%%%%%%%%%%%%%%%%%%%%%%%%%%%%%%%%%%%%%%%%%%%%%%%%%%%%%%%%%%%%%%%%%%%%%%%%%%%%%%%%%%%%%%%%%%%%%%%%%%%%%%%%%%%%%%%%%%%%%%%%%%%%%%%%%%%%
%%%%%%%%%%%%%%%%%%%%%%%%%%%%%%%%%%%%%%%%%%%%%%%%%%%%%%%%%%%%%%%%%%%%%%%%%%%%%%%%%%%%%%%%%%%%%%%%%%%%%%%%%%%%%%%%%%%%%%%%%%%%%%%%%%%%%%%%%%%%%%%%%%%%%%%%%%%%%%%%%%%%%%%%%%%%
\section{Solutions to exercises from chapter 5}

%%%%%%%%%%%%%%%%%%%%%%%%%%%%%%%%%%%%%%%%%%%%%%%%%%%%%%%%%%%%%%%%%%%%%%%%%%%%%%%%%%%%%%%%%%%%%%%%%%%%%%%%%%%%%%%%%%%%%%%%%%%%%%%%%%%%%%%%%%%%%%%%%%%%%%%%%%%%%%%%%%%%%%%%%%%%
%%%%%%%%%%%%%%%%%%%%%%%%%%%%%%%%%%%%%%%%%%%%%%%%%%%%%%%%%%%%%%%%%%%%%%%%%%%%%%%%%%%%%%%%%%%%%%%%%%%%%%%%%%%%%%%%%%%%%%%%%%%%%%%%%%%%%%%%%%%%%%%%%%%%%%%%%%%%%%%%%%%%%%%%%%%%
%%%%%%%%%%%%%%%%%%%%%%%%%%%%%%%%%%%%%%%%%%%%%%%%%%%%%%%%%%%%%%%%%%%%%%%%%%%%%%%%%%%%%%%%%%%%%%%%%%%%%%%%%%%%%%%%%%%%%%%%%%%%%%%%%%%%%%%%%%%%%%%%%%%%%%%%%%%%%%%%%%%%%%%%%%%%
\section{Solutions to exercises from chapter 6}
\paragraph{Exercise \ref{exer:contraction_TT_ss} (page \pageref{exer:contraction_TT_ss})}\mbox{}\\
\paragraph{Exercise \ref{exer:comm_delta_SUSY} (page \pageref{exer:comm_delta_SUSY})}\mbox{}\\
\paragraph{Exercise \ref{exer:beta_gamma_weight} (page \pageref{exer:beta_gamma_weight})}\mbox{}\\
\paragraph{Exercise \ref{exer:leading_term_OPE_TT_beta_gamma_system} (page \pageref{exer:leading_term_OPE_TT_beta_gamma_system})}\mbox{}\\
\paragraph{Exercise \ref{exer:comm_Q_b_beta} (page \pageref{exer:comm_Q_b_beta})}\mbox{}\\

%%%%%%%%%%%%%%%%%%%%%%%%%%%%%%%%%%%%%%%%%%%%%%%%%%%%%%%%%%%%%%%%%%%%%%%%%%%%%%%%%%%%%%%%%%%%%%%%%%%%%%%%%%%%%%%%%%%%%%%%%%%%%%%%%%%%%%%%%%%%%%%%%%%%%%%%%%%%%%%%%%%%%%%%%%%%
%%%%%%%%%%%%%%%%%%%%%%%%%%%%%%%%%%%%%%%%%%%%%%%%%%%%%%%%%%%%%%%%%%%%%%%%%%%%%%%%%%%%%%%%%%%%%%%%%%%%%%%%%%%%%%%%%%%%%%%%%%%%%%%%%%%%%%%%%%%%%%%%%%%%%%%%%%%%%%%%%%%%%%%%%%%%
%%%%%%%%%%%%%%%%%%%%%%%%%%%%%%%%%%%%%%%%%%%%%%%%%%%%%%%%%%%%%%%%%%%%%%%%%%%%%%%%%%%%%%%%%%%%%%%%%%%%%%%%%%%%%%%%%%%%%%%%%%%%%%%%%%%%%%%%%%%%%%%%%%%%%%%%%%%%%%%%%%%%%%%%%%%%
\section{Solutions to exercises from Appendix A}
\paragraph{Exercise \ref{exer:comm_psi_I_J_+_-} (page \pageref{exer:comm_psi_I_J_+_-})}\mbox{}\\
